# Supplementary material for: Uniform convergence of an upwind discontinuous Galerkin method for solving scaled discrete-ordinate radiative transfer equations with isotropic scattering kernel
Source: arXiv:2009.11356 source file (2020-09-23)
Supplement: Supplementary file 1 [file appendix_v6.tex]

\appendix

\section{Additional a priori estimates}
We provide here another two a priori estimates. 
First, inspired by \cite{ES2014}, we have the following lemma.
\begin{lemma}\label{lem:priori_est}
	Let $\bm{u}$ be the solution of \eqref{eq:rte_scale_compact} with $\bm{f}\in [L^2(X)]^L$ and $\bm{\alpha}\in [L^2(X)]^L$. Then
	\begin{equation}
	\|\bm{u}\|^2_{\partial X_+} + \frac{1}{\varepsilon}\|\bm{u}-\overline{\bm{u}}\|^2 + \varepsilon \|\overline{\bm{u}}\|^2
	\le C\left(\|\bm{\alpha}\|^2_{\partial X_-} + {\varepsilon}\|\overline{\bm{f}}\|^2 + \varepsilon^3\|\bm{f}-\overline{\bm{f}}\|^2\right),
	\end{equation}
	and
	\begin{equation}
	\varepsilon\|\bOmega\cdot\nabla\bm{u}-\overline{\bOmega\cdot\nabla\bm{u}}\|^2 + \frac{1}{\varepsilon}\|\overline{\bOmega\cdot\nabla\bm{u}}\|^2 + \|\bm{u}\|^2_{\partial X_+} \le C\left(\varepsilon\|\overline{\bm{f}}\|^2 +\varepsilon^3\|\bm{f}-\overline{\bm{f}}\|^2+\|\bm{\alpha}\|^2_{\partial X_-}\right),
	\end{equation}
	where $C$ only depends on the domain and the coefficients. 
\end{lemma}
\begin{remark}
	In the above lemma, $\bm{f}$ is not assumed to be isotropic. If $\bm{f}$ is isotropic, we have $\|\bm{f}-\overline{\bm{f}}\|=0$.
\end{remark}

\begin{corollary}\label{cor:well_posedness}
	In addition to the conditions in \cref{lem:priori_est}, assuming further that $\bm{\alpha}=O(\sqrt{\varepsilon})$, we have $\bm{u}\in \left[H^1(X)\right]^L$.
\end{corollary}

%Then we have the following estimate (cf. \cite{WY2015}).
%\begin{lemma}\label{lem:pri_3}
%	There is a constant $c$, uniform with respect to $\varepsilon$, so that
%	\begin{equation}\label{lem:priori_est_3}
%	\|\bm{u}\| \le c(\|\bm{\alpha}\|_{\partial X_-} + \varepsilon\|\bm{f}\| ).
%	\end{equation}
%\end{lemma}
%The proof of the above lemma can be divided into two steps. First step is to bound $\bm{u}-\overline{\bm{u}}$, which can be achieved also by employing \cref{lem:priori_est}. The more difficult step is to bound $\overline{\bm{u}}$. Interested readers can refer Lemma 3.4 in \cite{WY2015} for a proof for radiative transfer equations.
